# Supplementary material for: Relightable 3D Gaussians: Realistic Point Cloud Relighting with BRDF Decomposition and Ray Tracing
Source: arXiv:2311.16043 source file (2024-08-08)
Supplement: Supplementary file 1 [file X_supp.tex]

\section{Performance on Real-World Data}
\label{sec:supp_result}
We additionally assess Novel View Synthesis (NVS) on Real-World Data through both quantitative and qualitative analyses. Specifically, we compare our approach with previous inverse rendering methods on the real-world DTU dataset. It should be mentioned that our method utilizes masks from~\cite{yariv2020multiview}. And, we employ SfM points from COLMAP to initialize the 3D Gaussians. The results are depicted in Table~\ref{tab:exp_dtu} and Figure~\ref{fig:baselines}. The experiment reveals that our method achieves improved NVS accuracy on average. Furthermore, the visualizations illustrate that our approach excels in providing finer details.

\input{figs/baselines}
\input{figs/geometry}
\input{table/dtu}

\section{Geometry Enhancement}
\label{sec:supp_geometry}
3D Gaussian Splatting (3DGS)~\cite{kerbl20233d} demonstrates its advantages in fast training and real-time high-quality rendering. However, it struggles with accurate geometry recovery due to the Shape-Radiance Ambiguity~\cite{zhang2020nerf++}, as depicted in Fig~\ref{fig:geometry}. Specially, we convert the rendered depth maps of 3DGS to normal maps for visualization. 

Due to insufficient constraints, unexpected 3D ellipsoids appear in depth maps generated by 3DGS on the DTU dataset. For better visualization, the 3DGS normal maps of Scan105 and Scan108 in Fig. are post-processed using the masks from ~\cite{yariv2020multiview}. Since our method incorporates object masks as constraints, such a post-processing is not necessary. Comparison in Fig.~\ref{fig:geometry} reveals that our method significantly enhances the geometric quality of 3DGS, as evidenced by the visual improvements. It's worth noting that we solely relied on real observed images \textbf{without} any additional supervision, such as monocular depth or MVS depth.

Furthermore, as shown in Fig~\ref{fig:geo_albation}, we conduct a detailed ablation study on our proposed geometry enhancement, including \textbf{Constraint on Depth Distribution} and \textbf{Normal Gradient Based Densification}. The inclusion of the constraint on depth distribution aids in reducing uncertainty of depth, significantly contributing to our method's geometric enhancement. Additionally, the incorporation of densification based on normal gradient results in visually appealing details in the normal map.

\input{figs/geo_albation}

\section{Scenes Composition and Relighting} 
\label{sec:supp_relighting}
We present results showcasing relighting in multi-object composition scenes in Fig.~\ref{figs:nerf_composition}. For further insights into the comprehensive demonstration, we highly encourage referring to \textbf{our supplementary video}.

\input{figs/nerf_composition}
